# Supplementary material for: Neural basis expansion analysis with exogenous variables: Forecasting electricity prices with NBEATSx
Source: arXiv:2104.05522 source file (2022-04-04)
Supplement: Supplementary file 1 [file variance_decomposition.tex]

%================================================================================================
% VARIANCE DECOMPOSITION
%================================================================================================

\subsection{Week-long Hourly Electricity Price Decomposition}

By simply varying the dimensionality of the model's output $H$, we can apply NBEATSx to forecast over short or long horizons, or as an interpolation or extrapolation tool, according to the user's needs. Figure \ref{fig:variance_decomposition} shows the NP electricity market's hourly price, in Euros per megawatt, from May 28, 2013 to June 03, 2013, and the interpretable NBEATSx-I based decomposition from top to bottom: the first panel shows the original time series for the chosen week and the level, that corresponds to the last available value before the prediction; the second panel shows the inferred trend component, the third panel shows the seasonal component, the fourth panel exhibits the effects of exogenous covariates, and the last panel tracks the forecast residuals that can provide useful insights to detect unexpected variations of the signal. 
The data shows a minor effect of the trend, an evident seasonal effect within the days, and the system load effects with its weekend interactions identified by the model through the exogenous component. This example shows how the seasonal covariates can help NBEATSx identify longer seasonal effects than those included in the backcast period.

\begin{figure}[tbp]
\centering
\includegraphics[width=.90\linewidth]{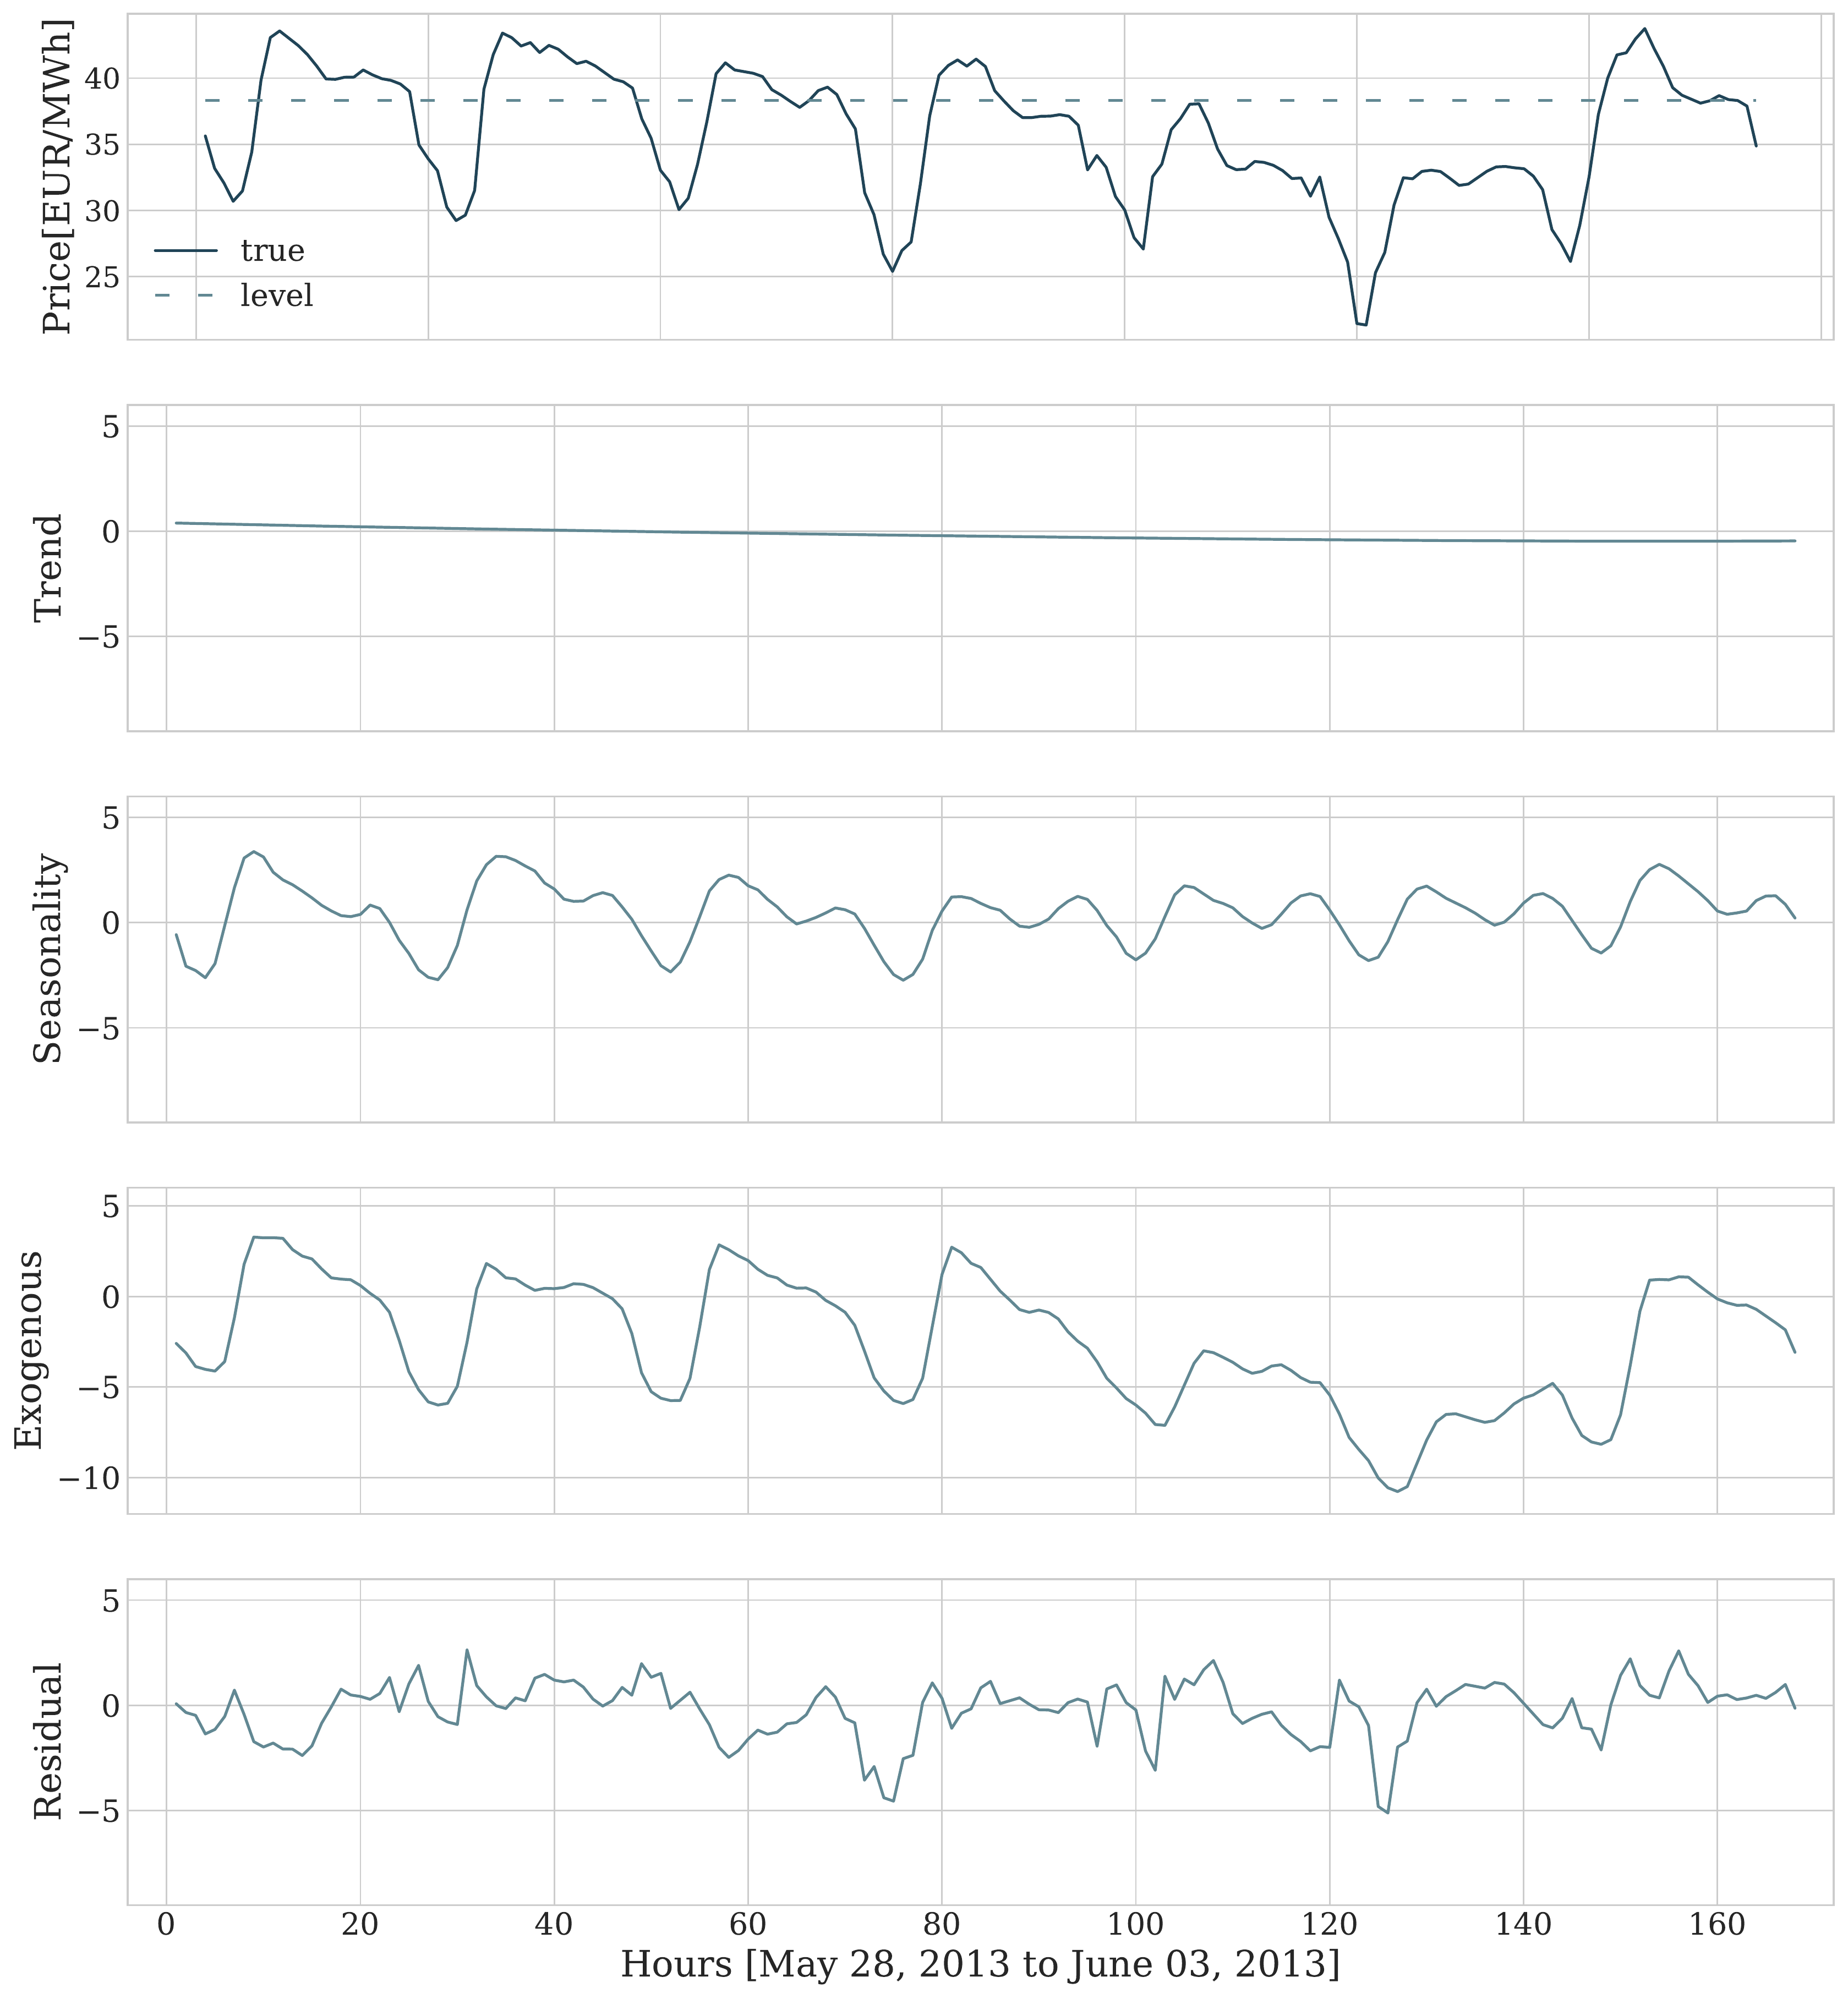}
\caption{NP electricity price week-ahead forecast decomposed using the interpretable NBEATSx. The top graph shows the original signal and the level, the latter is defined as the last available observation before the forecast, the second row corresponds to the polynomial trend, the third and fourth graphs display complex seasonality modeled by non linear Fourier projections and the exogenous effects of the electricity load on the price, and the final panel depicts the unexplained variation of the signal.} \label{fig:variance_decomposition}
\end{figure}
